# Supplementary material for: Lighter-X: An Efficient and Plug-and-play Strategy for Graph-based Recommendation through Decoupled Propagation
Source: arXiv:2510.10105 source file (2025-10-11)
Supplement: Supplementary file 1 [file appendix_future.tex]

\section{Other Related Works and Future Direction}
\label{sec:future}

\subsection{General Recommendation with Graph Side Information}
Traditional recommender systems only utilize interactions to model users' preferences for items. However, there is often graph-structured side information in recommendation scenarios, such as social networks between users and knowledge graphs associated with items~\cite{wu2022survey_gnnrec}. Several studies have introduced social networks or knowledge graphs into the design of recommendation models to improve performance further.

In general, social networks only contain information about whether users are friends, but the strength of the social relationships is usually unknown. To aggregate information from friends, it is necessary to determine the influence of neighbors. DiffNet~\cite{wu2019diffnet} utilizes a mean pooling operation to treat the influence of friends equally. However, the assumption of equal influence is untrue, as a user's influence should not be simply determined by the number of their friends. In fact, users are more likely to follow friends who have close relationships or similar preferences. Therefore, the attention mechanism is widely used to differentiate the influence of neighbors~\cite{wu2020diffnet++, fan2019socialrec, song2019session_social}.

Similarly, knowledge graphs utilize attributes to represent diverse relationships between items, which can improve the representativeness of items. The intuition behind is that items purchased by users often exhibit relational interconnections. For example, users often buy items from the same brand or origin. Therefore, KGAT~\cite{wang2019kgat}, TKGAT~\cite{wang2022tkgat}, and KGIN~\cite{wang2021kgin} consider users as a distinct type of entity and interpret interactions between users and items as relational links. This effectively integrates the user-item bipartite graph into the overall knowledge graph, enabling joint embedding learning from a unified heterogeneous graph structure. Additionally, models such as KQGC~\cite{kikuta2022kqgc} and KGCN~\cite{wang2019kgcn} treat users as queries for assigning weights to different relationships, accentuating the user's preference for items.

Incorporating side information densifies the originally sparse user-item bipartite graph~\cite{wu2022survey_gnnrec}. Since we do not modify the way of modeling graphs or the message passing mechanism, our method remains applicable for reducing parameters when the input consists only of user and item IDs. When using the attribute information of users and items as inputs, these attributes can replace the random initialization matrix in our method and be used as input features. Therefore, the proposed method is widely applicable to scenarios where only ID inputs are used, as well as to scenarios where additional attribute data are fused.

\subsection{GNNs for Sequential Recommendation}
Sequential recommendation mines sequential patterns between consecutively interacted items, aiming to predict a user's next preference based on their recent activity history~\cite{gao2023survey_gnnrec}. The sequential adjacencies between items are typically modeled as a graph structure, where each user's interaction sequence is transformed into a sequence graph. The most straightforward approach is to construct the graph with items as nodes and directed edges between successive interacted items~\cite{gupta2021causer, pan2020stargnn, gupta2019niser, wu2019sessionrec}. However, since most user sequences are short, a common technique is to enrich the item-item transitions using additional sequences. These can include different kinds of behavioral sequences~\cite{yang2022multibehavior}, historical sequences of the same users~\cite{zhang2020personalized}, or similar sequences in the full dataset~\cite{zhou2021temporal_sessionrec, wang2020global}. Augmenting the graphs with supplementary sequences helps densify the sparse item-item transitions to capture sequential relationships better~\cite{wu2022survey_gnnrec}. This graph densification enables more effective sequential modeling, especially when user sequences are inadequate to learn robust sequence-aware representations.

Since user and item IDs are the only inputs used in sequential recommendation, the proposed method appears to be capable of parameter reduction. However, the data is constructed into sequence subgraphs rather than a complete graph structure, and aggregation is performed selectively rather than on a full interaction or adjacency matrix. In order to match the formulation of distinct sequence graphs, the computations need to be modified. Specifically, the method for reducing parameters would require customization to accommodate the neighborhood aggregation and localized message passing that occur within sequence graphs. The fundamental ideas of pre-computing propagations and simplifying feature transformations are still applicable, but their precise application depends on the given sequence-aware purpose and the manner of modeling graphs. This is an interesting direction we aim to explore in future work.
